# Supplementary material for: Discovering New Strong Gravitational Lenses in the DESI Legacy Imaging Surveys
Source: arXiv:2005.04730 source file (2021-01-10)
Supplement: Supplementary file 1 [file appendix-data.tex]

%% Appendix B
\setcounter{figure}{0}
Possibly something here.
